# Supplementary material for: Fragment, Entangle, and Consolidate: Strong Correlation through Bi-fold Quantum Circuits
Source: arXiv:2510.15678 ancillary file (2025-10-17)
Supplement: Supplementary file 1 [file Supplementary_Information.pdf]

# Supplementary information: Fragment, Entangle, and Consolidate: Strong Correlation through Bi-fold Quantum Circuits

Arpan Choudhury,[†,¶] Sonaldeep Halder,[‡,¶] Rahul Maitra,[*,‡] and Debashree Ghosh[*,†]

†*School of Chemical Sciences, Indian Association for the Cultivation of Science, Kolkata, India*

‡*Department of Chemistry, IIT Bombay, Mumbai, India*

¶*These authors contributed equally.*

E-mail: rmaitra@chem.iitb.ac.in; pcdg@iacs.res.in

## Section S1: Qubit-ADAPT-VQE

In the fermionic-ADAPT-VQE protocol, it remains uncertain how many operators should be included in the operator pool and whether the pool is complete enough to ensure convergence to the ground state energy. An alternate way to construct a new operator pool is to break down the fermionic excitations into individual Pauli strings after the Jordan-Wigner (JW) mapping. The exponentials of fermionic excitation operators, when mapped via the JW transformation, are represented in terms of quantum gates as

$$e^{\theta_i^a \hat{\tau}_i^a} = \exp\Big[\mathrm{i}\frac{\theta_i^a}{2} \prod_{k=i+1}^{a-1} Z_k \ \ \big(X_a Y_i - Y_a X_i\big)\Big], \tag{1}$$

$$\begin{aligned} e^{\theta_{ij}^{ab} \hat{\tau}_{ij}^{ab}} = \exp\Big[\mathrm{i}\frac{\theta_{ij}^{ab}}{8} \prod_{k=i+1}^{j-1} Z_k \ \prod_{l=a+1}^{b-1} Z_l \ \ \big(&X_a Y_b X_i X_j + Y_a X_b X_i X_j + Y_a Y_b Y_i X_j + Y_a Y_b X_i Y_j \\ &- X_a X_b Y_i X_j - X_a X_b X_i Y_j - Y_a X_b Y_i Y_j - X_a Y_b Y_i Y_j\big)\Big]. \end{aligned} \tag{2}$$

From Eq. 1 and 2, we can see that any pair of Pauli strings differs by only an even number of Pauli operators there are only an odd number of $X$ and $Y$ gates in the Pauli strings. This implies that the individual Pauli strings commute with one another and therefore commute with each other. Thus, the exponential of fermionic excitation operators can be written as a product of exponentials of individual Pauli strings

$$e^{\theta\hat{\tau}} = \prod_k e^{\mathrm{i}\theta \hat{P}_k}, \tag{3}$$

where the Pauli strings $\hat{P}_k = \prod_n p_n$ , $p_n \in \{X, Y, Z\}$. In the qubit-ADAPT protocol, these Pauli strings form the operator pool instead of the fermionic excitations and are added to the ansatz iteratively.

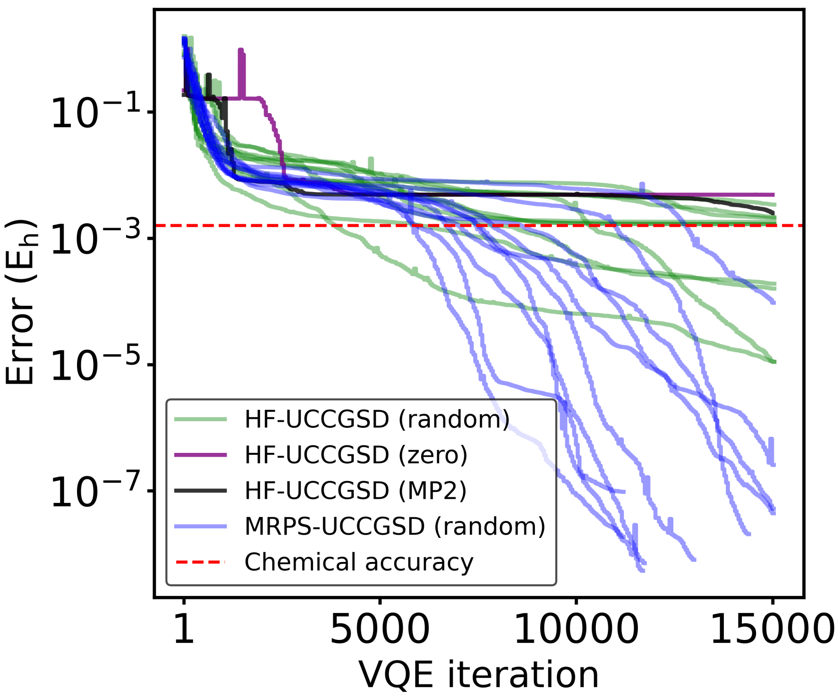


Fig S1. Error in energy (in Hartree) for UCCGSD simulations of the square $H_4$ system using MRPS reference state (with random initial parameters), and HF reference state (with random, zero and MP2 initial parameters) against the VQE iteration.

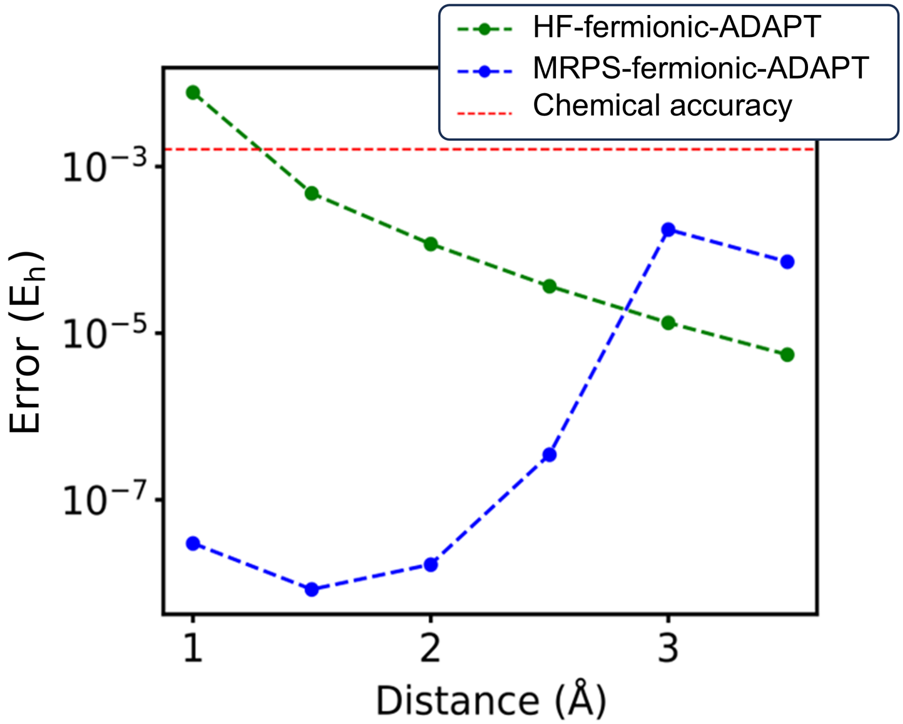


Fig S2. Error (in Hartree) in the potential energy curve of the $H_4$ molecule by changing the $r_2$ distance while keeping the $r_1$ distance fixed at 1.0 Å. HF-fermionic-ADAPT-VQE and MRPS-fermionic-ADAPT-VQE refer to the ADAPT-VQE using operator pool consisting of fermionic singles and doubles excitations, and starting with HF and MRPS initial states, respectively.

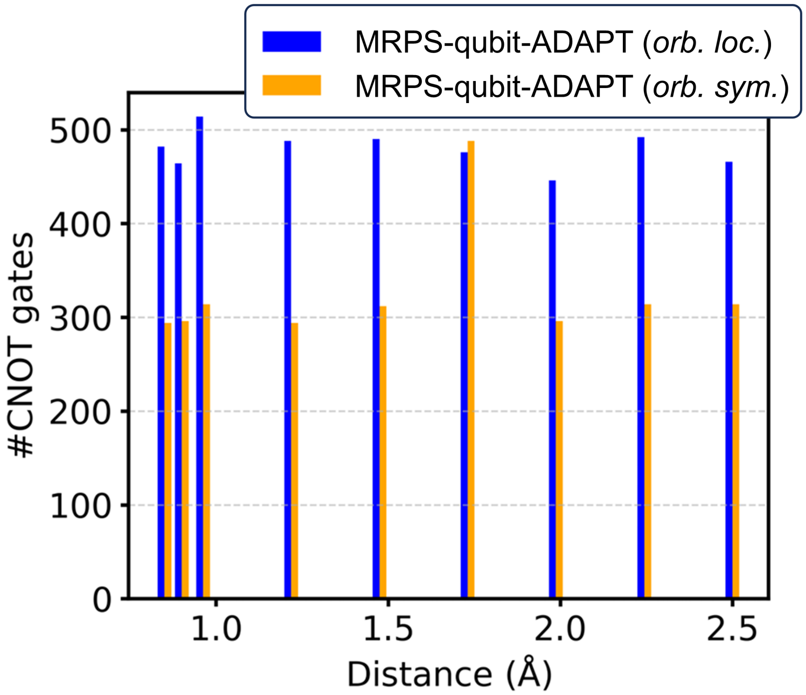


Fig S3. Number of CNOT gates required by the MRPS-qubit-ADAPT-VQE method for calculating the potential energy curve for double dissociation of two O–H bonds in water molecule. The fragment states are prepared based on orbital locaization as well as orbital symmetries.

Table S1: Fidelity between the prepared and exact fragment state with the number of layers in the HEA using linear entanglement blocks.

| Layer | $H_4$ rectangular | $H_4$ square | CBD ($D_{2h}$) | CBD ($D_{4h}$) |
|---|---|---|---|---|
| 1 | 0.9978 | 0.9707 | 0.9566 | 0.9914 |
| 2 | 0.9999 | 0.9789 | 0.9999 | 0.9999 |
| 3 | 0.9999 | 0.9999 | 0.9999 | 0.9999 |
| 4 | 0.9999 | 0.9999 | 0.9999 | 0.9999 |
| 5 | 0.9999 | 0.9999 | 0.9999 | 0.9999 |
| 6 | 0.9999 | 0.9999 | 0.9999 | 0.9999 |
| 7 | 0.9999 | 0.9999 | 0.9999 | 0.9999 |
| 8 | 0.9999 | 0.9999 | 0.9999 | 0.9999 |
